# Supplementary material for: Phase separation of active Brownian particles on curved surfaces
Source: arXiv:2212.08561 source file (2022-12-16)
Supplement: Supplementary file 1 [file supplementary.pdf]

# Supplementary Information for
# Phase separation of active Brownian particles on curved surfaces

Priyanka Iyer, Roland G. Winkler, Dmitry A. Fedosov, and Gerhard Gompper*

(Dated: December 16, 2022)

## I. ANALYTICAL SOLUTION OF THE LANGEVIN EQUATION FOR ABPS ON A RING

The equation of motion for an active Brownian particle (ABP) with a position vector $\mathbf{r} = R(\cos\theta, \sin\theta)$, orientation vector $\mathbf{e} = (\cos\psi, \sin\psi)$, confined to move on a ring with radius $R$ in two dimensions (2D), is given by

$$\begin{aligned}\dot{\mathbf{r}} &= v_0(\mathbf{e}\cdot\mathbf{e}_\theta)\mathbf{e}_\theta, \quad \dot{\theta} = -\frac{v_0}{R}\sin(\theta-\psi),\\ \dot{\psi} &= \sqrt{2D_r}\Gamma_\psi,\end{aligned} \tag{1}$$

where $v_0$ is the ABP propulsion velocity, $\mathbf{e}_\theta = \mathbf{r}/R$, $D_r$ is the rotational diffusion, and $\Gamma_\psi$ is the rotational noise with $\langle\Gamma_\psi\rangle = 0$ and $\langle\Gamma_\psi(t)\Gamma_\psi(t')\rangle = \delta(t-t')$. After the linearization of these equations in the limit of large Pe (i.e., small misalignment angle $|\delta| \equiv |\theta-\psi| \ll 1$) and normalization of time by $\tau = R/v_0$, we obtain the dimensionless equations

$$\dot{\theta} = -\theta + \psi, \quad \dot{\psi} = \tau\sqrt{2D_r}\Gamma_\psi, \tag{2}$$

$$\ddot{\theta} = -\dot{\theta} + \tau\sqrt{2D_r}\Gamma_\psi. \tag{3}$$

The Fokker-Plank equation for $\dot{\theta}$ is given by

$$\frac{\partial}{\partial t^*}P(\dot{\theta}, t^*) = \frac{\partial}{\partial\dot{\theta}}(\dot{\theta}P(\dot{\theta}, t^*)) + D_r\tau\frac{\partial^2}{\partial\dot{\theta}^2}P(\dot{\theta}, t^*) \tag{4}$$

where $t^*$ denotes the dimensionless time. In the stationary state, we obtain

$$P(\dot{\theta}) = \frac{1}{\sqrt{2\pi D_r\tau}}\exp\left[\frac{-\dot{\theta}^2}{2D_r\tau}\right], \quad \langle\dot{\theta}^2\rangle = D_r\tau. \tag{5}$$

Integration of Eq. (3) leads to

$$\begin{aligned}\dot{\theta}(t^*) &= \dot{\theta}(0)e^{-t^*} + \tau e^{-t^*}\int_0^{t^*}\sqrt{2D_r}\Gamma_\psi(s)e^s ds,\\ \langle\dot{\theta}(t_1^*)\dot{\theta}(t_2^*)\rangle &= \dot{\theta}^2(0)e^{-(t_1^*+t_2^*)} + \tau D_r[e^{-|t_1^*-t_2^*|} - e^{-(t_1^*+t_2^*)}].\end{aligned} \tag{6}$$

Then, the angular mean-squared displacement (MSD) can be calculated using $\theta(t^*) - \theta(0) = \int_0^{t^*}\dot{\theta}(s)ds$, and is given by

$$\begin{aligned}\langle(\theta(t^*) - \theta(0))^2\rangle &= \int_0^{t^*}\int_0^{t^*}\langle\dot{\theta}(s')\dot{\theta}(s)\rangle ds ds' =\\ &= (\dot{\theta}^2(0) - \tau D_r)(1-e^{t^*})^2 + 2\tau D_r t^* - 2(1-e^{-t^*})\tau D_r.\end{aligned} \tag{7}$$

Finally, using the result $\langle\dot{\theta}^2\rangle = \tau D_r$ from Eq. (5), we obtain

$$\langle(\theta(t^*) - \theta(0))^2\rangle = 2\tau D_r t^* - 2(1-e^{-t^*})\tau D_r. \tag{8}$$

MSD in the dimensional form becomes

$$\langle(\theta(t) - \theta(0))^2\rangle = 2D_r t - 2\tau D_r[1 - \exp(t/\tau)], \tag{9}$$

and in the limit of small and large times, MSD is given by

$$\langle(\theta(t) - \theta(0))^2\rangle = \begin{cases}(\tau_r\tau)^{-1}t^2, & t\to 0,\\ 2D_r t, & t\to\infty,\end{cases} \tag{10}$$

where $\tau_r = D_r^{-1}$ is the rotational diffusion time and $\langle\dot{\theta}^2\rangle = (\tau_r\tau)^{-1}$. Therefore, the transition from ballistic to diffusive motion takes place at $t \sim \tau$, suggesting that for large curvatures (or small $R$), the particle moves ballistically for times shorter than $\tau = R/v_0$.

For the misalignment angle $\delta = \theta - \psi$, we have the dimensionless equation

$$\dot{\delta} = -\sin\delta + \tau\sqrt{2D_r}\Gamma_\psi, \tag{11}$$

with the corresponding Fokker-Planck equation

$$\frac{\partial}{\partial t^*}P(\delta, t^*) = \frac{\partial}{\partial\delta}[(\sin\delta)P(\delta, t^*))] + \tau D_r\frac{\partial^2}{\partial\delta^2}P(\delta, t^*). \tag{12}$$

Equation (12) can be solved to obtain the stationary-state distribution

$$P(\delta) = \frac{1}{2\pi I_0(\tau_r/\tau)}\exp\left[\frac{\cos\delta}{\tau D_r}\right], \tag{13}$$

where $I_0(\tau_r/\tau)$ is the modified Bessel function of the first kind. In the limit $|\delta| \ll 1$, $\dot{\theta} = \delta$, and the resulting distributions for $\delta$ and $\dot{\theta}$ are identical and given in Eq. (5). In the limit $|\delta| \ll 1$, the dimensional tangential velocity $v = v_0\sin\delta$ becomes

$$\sqrt{\langle v^2\rangle} = v_0\sqrt{\tau/\tau_r}, \tag{14}$$

* Theoretical Physics of Living Matter, Institute of Biological Information Processing and Institute for Advanced Simulation, Forschungszentrum Jülich, 52425 Jülich, Germany
Email: p.iyer@fz-juelich.de, r.winkler@fz-juelich.de, d.fedosov@fz-juelich.de, g.gompper@fz-juelich.de

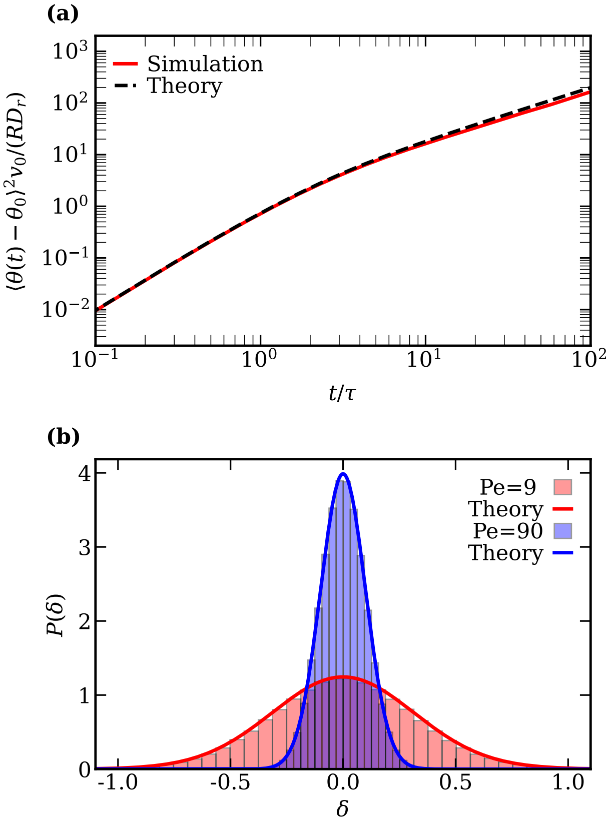


FIG. S1: (a) Angular MSD of a single particle confined to move on a ring in 2D. The MSD shows an initial ballistic regime, followed by long-time diffusive behaviour. The crossover time is given by $\tau = R/v_0$. (b) Distribution of the misalignment angle $\delta = \theta - \psi$ as a function of Pe. The lines represent theory, and the histograms are obtained from simulations. The distribution becomes narrower with increasing Pe, leading to smaller fluctuations of the misalignment angle, and therefore, a lower tangential velocity.

where we have used that $\langle \delta^2 \rangle = \tau/\tau_r$. Thus, the particle tangential velocity decreases with both increasing activity (equivalently increasing $\tau_r$) and increasing curvature (or decreasing $\tau$). Figure S1 shows a comparison of the MSD and distribution of the misalignment angle from the linearized theory and the corresponding simulations.

## II. SIMULATION METHODS

Self-propelled particles are simulated as active Brownian particles (ABPs) embedded in three dimensions (3D) but restricted to move on a 2D spherical surface. An ABP experiences a propulsion force $f_p$ acting along its orientation vector $\mathbf{e}_i$. The equation of motion for the position $\mathbf{r}_i$ of an APB is given by

$$m\ddot{\mathbf{r}}_i = f_p \mathbf{e}_i - \gamma \dot{\mathbf{r}}_i - \nabla_i (U_{\rm conf} + U_{\rm int}), \tag{15}$$

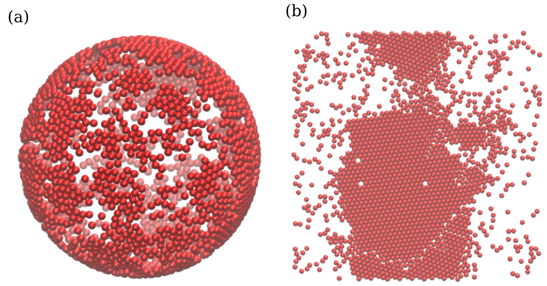


FIG. S2: Simulation snapshots for a fixed Pe = 890 and $\phi = 0.5$. (a) Spherical geometry with $R/\sigma = 16.1$ and $N = 2074$, and (b) planar confinement ($R = \infty$) with $N = 1834$. The two systems have nearly same number of particles, indicating that the absence of MIPS for $R/\sigma = 16.1$ is not predominantly due to finite-size effects.

where $m$ is the particle mass, $\gamma$ is the friction coefficient, $U_{\rm conf}$ is the confinement potential for ABPs, $U_{\rm int}$ is the pair-wise interaction potential between different ABPs, and $\nabla_i$ is the spatial derivative at particle $i$. The orientation vector $\mathbf{e}_i$ is subject to a diffusive rotation modeled as

$$\dot{\boldsymbol{e}}_i = \boldsymbol{\zeta}_i \times \boldsymbol{e}_i, \tag{16}$$

where $\boldsymbol{\zeta}_i$ is a Gaussian random process with $\langle \boldsymbol{\zeta}_i(t) \rangle = 0$ and $\langle \boldsymbol{\zeta}_i(t) \boldsymbol{\zeta}_j(t') \rangle = 2D_{\rm r} \delta_{ij} \delta(t-t')$ with a rotational diffusion coefficient $D_{\rm r}$. Note that we neglect the effect of translational noise in Eq. (15). The confinement and particle-particle interactions are represented by the Lennard-Jones (LJ) potential as

$$U(r) = \begin{cases} 4\epsilon \left[ \left(\frac{\sigma_{LJ}}{r}\right)^{12} - \left(\frac{\sigma_{LJ}}{r}\right)^{6} \right], & \text{if } r < r_c, \\ 0, & \text{if } r \geq r_c, \end{cases} \tag{17}$$

where $\sigma_{LJ}$ is the distance at which $U(\sigma_{LJ}) = 0$ and $\epsilon$ is the potential strength. For the confinement interactions, the cutoff radius is set to $r_c = 2^{1/6}\sigma_{LJ}/2$, while for the ABP-ABP interactions, $r_c = 2^{1/6}\sigma_{LJ}$, so that only repulsive (no attraction) interactions between particles are considered. Confinement of the ABPs to a 2D spherical surface of radius $R$ is achieved by placing two concentric spherical surfaces with radii $R + \sigma_{LJ}/2$ and $R - \sigma_{LJ}/2$, at which the LJ potential is applied.

Activity of the ABPs is described by the dimensionless Péclet number $\text{Pe} = f_p/(\gamma\sigma D_r) = v_0\tau_r/\sigma$, where $\sigma = 2^{1/6}\sigma_{LJ}$ is the ABP diameter. The surface density of the ABPs on a sphere is given by $\phi = N\sigma^2/(16R^2)$, where N is the total number of ABPs.

## III. PLANAR SIMULATIONS

To study the finite-size effects due to a finite number $N$ of particles for a spherical confinement, we also perform simulations of ABPs moving in a planar (slit-like) geometry. This is achieved by confining the particles to the

x-y plane using two planar surfaces placed at $z = \sigma_{LJ}/2$ and $z = -\sigma_{LJ}/2$, at which the LJ potential is applied. In the x and y directions, periodic boundary conditions are employed. The simulation domain corresponds to a square with a side length $L$, where the surface density of ABPs is given by $\phi = N\pi\sigma^2/(4L^2)$. The corresponding simulation on a sphere has the same $N$ and $\phi$ with a sphere radius of $R/\sigma = L/(2\sqrt{\pi}\sigma)$.

Finite-size effects lead to a shift of the critical Péclet number $\mathrm{Pe}_c$ for motility-induced phase separation (MIPS) toward larger Pe values for decreasing $L$ (or $R$), see Fig. 3(b) in the main text. Thus, the boundary for MIPS in Fig. 3(b) of the main text representing $\mathrm{Pe}_c$ as a function of $R$ is corrected for finite-size effects measured in the planar simulations. Furthermore, to compare the effective Péclet number $\mathrm{Pe}_{eff}$ on a sphere with that for the planar case, we also compute the planar Péclet number $\mathrm{Pe}_{pl}$ based on the average mean-squared planar velocity $v$, i.e. $\mathrm{Pe}_{pl} = \mathrm{Pe}\sqrt{\langle v^2\rangle}/v_0$. For example, MIPS for $\phi = 0.5$ is first observed at $\mathrm{Pe} = 31$, which corresponds to $\mathrm{Pe}_{pl} \simeq 25$.

Figure S2 shows the simulation snapshots of ABPs on a sphere with radius $R/\sigma = 16.1$ and confined to a plane ($R = \infty$) at $\mathrm{Pe} = 890$. Both simulations have nearly same number of particles, however, MIPS is not observed on the sphere, indicating that the absence of MIPS for small spheres is indeed a curvature effect.

## IV. LOCAL DENSITY MEASUREMENTS

Two different methods are employed for local density measurements: (i) direct sampling of local density, and (ii) the construction of a Voronoi diagram. In the first method, a sampling grid of $N_s$ points is considered, and the local density for each sampling point $j$ at the position $\mathbf{s}_j$ is calculated as

$$\phi_{loc,j} = \pi\sigma^2 \frac{n_j^{\mathrm{p}}}{4A_{loc}}, \tag{18}$$

where $n_j^{\mathrm{p}}$ is the number of ABPs within the cutoff distance $r_{cut} = 4.5\sigma$ from the position $\mathbf{s}_j$ and $A_{loc} = \pi r_{cut}^2$ is the local area around each sampling point. This method is used for determining the co-existing densities in the phase separated state, as a uniform placement of sampling points ensures that the two peaks in local density are well separated and can easily be localized [see Fig. S3(a)].

The second method involves the construction of a Voronoi diagram given the particle positions as the generating points. After the Voronoi diagram is built, the area $A_i$ of each Voronoi cell associated with a particle $i$ is used to determine the local area as

$$\phi_{loc,i} = \pi\sigma^2/(4A_i). \tag{19}$$

In this method, the peak in local density representing the gas phase is low in intensity and broad due to a large variation in polygon areas for the low density state. On the other hand, the high density phase often exhibits multiple peaks, corresponding to variations in local ordering in the large MIPS cluster (locally crystalline, locally hexatic, and locally liquid). However, these local variations do not give a proper measure of the average local density in the MIPS cluster. This is why the local sampling method is used for the determination of co-existing densities. However, the Voronoi analysis can be performed much faster and does not depend on the choice of the cutoff distance $r_{cut}$, whose selection becomes increasingly harder as the system size decreases for decreasing $R$. As a result, both methods are employed in the analysis of MIPS, as they show the shift from uni-modal to bi-modal distribution of local density near the same (critical) Pe.

## V. PRESSURE MEASUREMENTS

Pressure in the simulated system is calculated using the virial theorem [1–3], which states that for a confined system of $N$ particles in the over-damped limit, we have

$$\sum_{i=1}^{N} \langle \mathbf{F}_i(t) \cdot \mathbf{r}_i(t) \rangle = 0, \tag{20}$$

where $\mathbf{F}_i(t)$ is the total force acting on particle $i$. Equation (20) is expanded by considering different forces present in the simulated system as

$$\sum_{i=1}^{N} \langle f_p e_i(t) \cdot \mathbf{r}_i(t) \rangle + \frac{1}{2} \sum_{i=1}^{N} \sum_{j=1}^{N} \langle \mathbf{F}_{i,j}(t) \cdot (\mathbf{r}_i(t) - \mathbf{r}_j(t)) \rangle + \sum_{i=1}^{N} \langle \mathbf{F}_{i,\mathrm{conf}}(t) \cdot \mathbf{r}_i(t) \rangle = 0, \tag{21}$$

where $\mathbf{F}_{i,\mathrm{conf}}(t)$ is the confinement force on particle $i$, and $\mathbf{F}_{i,j}(t)$ is the inter-ABP force between particles $i$ and $j$. Now, the internal virial $V_{\mathrm{int}}$ due to internal forces and the external virial $V_{\mathrm{ext}}$ due to forces from the confining potential can be defined as

$$\begin{aligned} V_{\mathrm{int}} &= \sum_{i=1}^{N} \langle f_p e_i(t) \cdot \mathbf{r}_i(t) \rangle \\ &\quad + \frac{1}{2} \sum_{i=1}^{N} \sum_{j=1}^{N} \langle \mathbf{F}_{i,j}(t) \cdot (\mathbf{r}_i(t) - \mathbf{r}_j(t)) \rangle, \\ V_{\mathrm{ext}} &= \sum_{i=1}^{N} \langle \mathbf{F}_{i,\mathrm{conf}}(t) \cdot \mathbf{r}_i(t) \rangle, \end{aligned} \tag{22}$$

where $V_{\mathrm{ext}} = -V_{\mathrm{int}}$. Then, the pressure in the system is related to the internal virial as

$$3pV \simeq V_{\mathrm{ext}} = -V_{\mathrm{int}}, \tag{23}$$

where $V = 4\pi R^2\sigma$. Thus, the pressure can be calculated using either the internal or external virial. In our

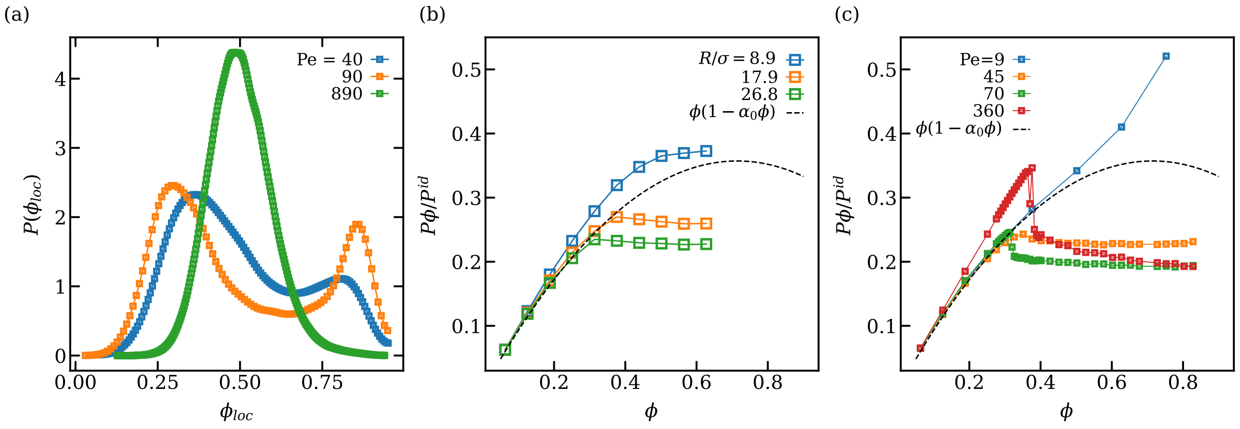


FIG. S3: (a) Local density distribution for different Pe at $R/\sigma = 16.1$ and $\phi = 0.5$. Note that at very large Pe, MIPS is lost and the distribution has a single peak at the mean density. (b) Pressure as a function of surface density for various $R$ at a fixed Pe $= 45$. The effect of decreasing $R$ is qualitatively similar to that of decreasing Pe. (c) Pressure as a function of surface density for different Pe at a fixed $R/\sigma = 26.8$. At the MIPS transition, a sudden drop in pressure is observed, which is more pronounced at large Pe. Also, at very large Pe, the $\phi$ value at the pressure drop stars increasing, in agreement with the observations of the local density measurements. The black dashed line is quadratic fit with $\alpha_0 = 0.7$.

simulation setup, the particles continuously interact with the 'confining' wall, and therefore, even $V_{\text{ext}}$ gives a good estimate of the system pressure due to sufficient averaging [see Fig. S3(b),(c)]. We have verified the equality $V_{\text{ext}} = -V_{\text{int}}$ for a few simulations. To compute pressure, the external virial is used for all simulations, as the computational cost of the external virial scales as $\sim N$, whereas for the internal virial, it scales as $\sim N^2$.

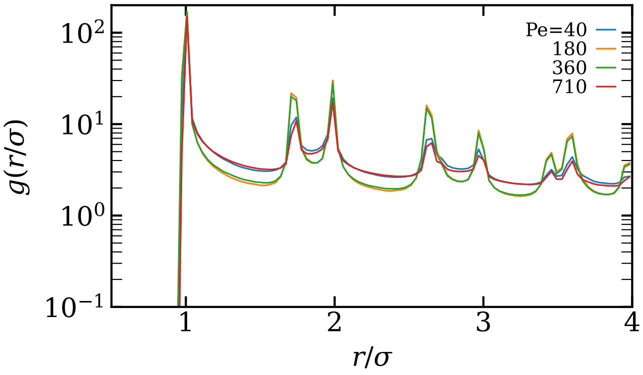


FIG. S4: Radial distribution function (RDF) of particles for different Pe at $R/\sigma = 16.1$. Location of the peaks is nearly independent of Pe, suggesting that the effective density is not altered. Moreover, the RDF for Pe $= 40$ is similar to that for Pe $= 710$, consistent with the observation of the 'turning' of the phase diagram at large Pe.

## VI. RADIAL DISTRIBUTION FUNCTION

Radial distribution function (RDF) of the particles is plotted in Fig. S4 for different Pe at $R/\sigma = 16.1$ in the phase separated state to check whether there is any change in the effective particle radii. RDFs for different Pe show no visible change in the peak positions, supporting that simulations do not suffer from any possible artifacts due to the softness of the particles. Therefore, the choice of ABP diameter as $\sigma = 2^{1/6}\sigma_{LJ}$ is well justified. Note that the peaks in RDF broaden for large Pe, suggesting that the effective Péclet number $\text{Pe}_{eff}$ on the sphere decreases at large Pe.

## VII. TWO CONNECTED SPHERES

To apply single-sphere results to a more complex system, we consider an ensemble of active particles moving on a surface of two connected spheres with different radii $R_1/\sigma = 16.1$ and $R_2 = 0.6R_1$. The simulation setup consists of two confining spheres of radii $R_1 + \sigma/2$ and $R_2 + \sigma/2$, with their centers at $(-R_1, 0, 0)$ and $(R_2 - \Delta, 0, 0)$, respectively, where $\Delta$ is the overlap of the two spheres in the x-direction (we set $\Delta = \sigma_{LJ}$). The corresponding two-pore surface applies the LJ potential to ABPs, in order to confine them inside. The LJ interaction is cut off at a distance $r_c = \sigma_{LJ}$ from the surface, so that only a single layer of ABPs is attracted to the surface. The intersection of the two spherical surfaces creates a region where particles may escape, as the normal is not well defined at the sharp boundary. Therefore, a neck of frozen particles interacting with the ABPs via the repulsive part of the LJ potential is placed at the intersection of two spheres to prevent the particles from escaping. The system is initiated with a homogeneous particle distribution on both spherical surfaces and is simulated for varying particle numbers and activity. Note that in this setup, ABPs may detach from the surface, as there is no inner confining surface which has been employed for the case of a single sphere. However, the occurrence of ABP detachment from the surface is very infrequent, and can be neglected, since the detached

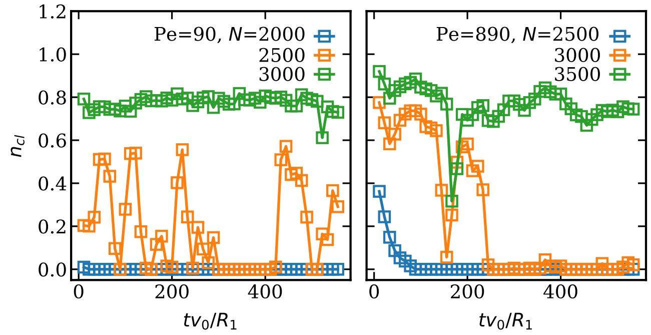


FIG. S5: Fraction $n_{cl}$ of particles occupying clusters of size larger than $N_1/2$ in the large sphere as a function of time for (a) Pe = 90 and (b) Pe = 890.

particles also very quickly reach the surface again.

Figure S5 shows the fraction $n_{cl}$ of particles occupying clusters of size greater than $N_1/2$ in the larger sphere as a function of time. Small $n_{cl}$ values imply that most of the formed clusters are small, whereas a large value of $n_{cl}$ indicates the formation of a large cluster, containing the majority of the particles (i.e., MIPS). A cutoff value of $1.1\sigma$ is used for the identification of ABP clusters. When the large sphere retains a sufficient number of particles, MIPS takes place, leading to large $n_{cl}$ values. Due to a low Pe$_{eff}$ at Pe = 890, a larger number of particles $N = 3500$ are required for MIPS in comparison to $N = 3000$ at Pe = 90, see the green curves in Fig. S5. For $N = 2500$ (Pe = 90) and $N = 3000$ (Pe = 890), the system is in an unstable regime where the MIPS state is dynamic. For Pe = 890 and $N = 3000$, there is an initial MIPS state in the larger sphere at small times followed by the disappearance of MIPS at times $tv_0/R_1 > 200$, see Fig. S5(b). This occurs because the larger sphere starts out with a sufficient number of particles for phase separation, but with time, loses particles to the smaller sphere. In this unstable regime, fluctuations in particle numbers within different pores are important and can lead to dynamic restoration and loss of MIPS, as can be seen in Fig. S5(a) where strong fluctuations in $n_{cl}$ for Pe = 90 and $N = 2500$ are present. Note that the fluctuations in ABP numbers within different pores are larger at a lower Pe.

## VIII. SUPPLEMENTARY MOVIES

**Movie S1**: Side-by-side simulations of ABPs on a sphere of radius $R/\sigma = 26.8$ and confined to a plane ($R/\sigma = \infty$) with $N = 5093$ and $N = 5760$, respectively. Both simulations have an area fraction of $\phi = 0.5$ and Pe=890. The largest cluster in both systems is colored in green, while all other ABPs are white. Both systems show MIPS.

**Movie S2**: Side-by-side simulations of ABPs on a sphere of radius $R/\sigma = 16.1$ and confined to a plane ($R/\sigma = \infty$) with $N = 2074$ and $N = 1834$, respectively. Both simulations have an area fraction of $\phi = 0.5$ and Pe=890. The largest cluster in both systems is colored in green, while all other ABPs are white. The particles in the sphere do no phase separate, as there are no clear high and low density phases (the largest cluster is spread across the sphere). On the other hand, the particles in the plane show MIPS.

**Movie S3**: Simulation of two connected pores with radii $R_1/\sigma = 16.1$ and $R_2/\sigma = 9.6$, N=2500, and Pe=90. The largest clusters in the larger and smaller spheres are colored red and green, respectively. The cluster in the larger sphere (red) is unstable, and dynamically shrinks and grows throughout the simulation.

[1] D. Levis, J. Codina, and I. Pagonabarraga, Active Brownian equation of state: metastability and phase coexistence, Soft Matter **13**, 8113 (2017).
[2] S. C. Takatori and J. F. Brady, Forces, stresses and the (thermo?) dynamics of active matter, Curr. Opin. Colloid Interface Sci. **21**, 24 (2016).
[3] R. G. Winkler, A. Wysocki, and G. Gompper, Virial pressure in systems of spherical active Brownian particles, Soft Matter **11**, 6680 (2015).
